# Supplementary material for: Event and Entity Extraction from Generated Video Captions
Source: arXiv:2211.02982 source file (2023-09-13)
Supplement: Supplementary file 1 [file 03_users_guide.tex]

\section{User's Guide}
\label{sec:users_guide}
This section describes how to use the implementation of our framework. In particular, we provide information on the installation of dependencies, and provide guidance on its usage.

\subsubsection*{Dense Video Captioning.}
Thanks to its modularity, any DVC models can be used for our framework. In this work, we make use of the MT \cite{MT} and PDVC \cite{PDVC} models. However, the source code that we provide for our framework does not include any implementation of the DVC models, mainly because the feature extraction of new videos, which are not contained in the ActivityNet Captions dataset, was not achieved with our hardware. Refer to the GitHub repositories MT\footnote{MT is available at: \url{https://github.com/salesforce/densecap}.} and PDVC\footnote{PDVC is available at: \url{https://github.com/ttengwang/PDVC}.} for the source code of the used DVC models and extensive information about their installation and usage. Furthermore, refer to Section~\ref{sec:experiments/hyperparameters} for the hyperparameters that we used for training MT and PDVC. For both models, we generated captioned events for ActivityNet Captions train and validation videos for $|E|$ set to 10, 25, 50, 100, and $|dist(E)|$ set to 1, 3, 10, 25 (i.e., the numbers of (distinct) captioned events). For each such configuration of DVC model and number of generated captioned events, a JSON file is created containing the results for all videos. These JSON files are then forwarded to the remaining components of the framework for the extraction of semantic metadata, and the evaluation of our framework.

\subsection*{Semantic Metadata Extraction}
The GitLab repository \texttt{2021ss-thesis-johannes} contains the source code for the extraction and evaluation of semantic metadata from captioned events and all necessary data files. We provide information on the installation of dependencies, as well as guidance on how to use the provided files to extract semantic metadata and evaluate our framework.

\subsubsection*{\textbf{Installation.}} \ \\
\noindent We recommend to use Anaconda\footnote{Anaconda is available at: \url{https://www.anaconda.com/}.} for package management. In order for the semantic metadata extraction methods to work, \texttt{python3} must be available. As mentioned in Section~\ref{sec:experiments}, we are bound to use version 2.3.7 within spaCy since NeuralCoref, a pipeline extension for spaCy which we use for coreference resolution, is not compatible with versions 3.0.0+ yet. After installation of Anaconda, run the following commands in the repository's root directory to install all necessary dependencies:

\vspace{1mm}
\begin{mdframed}[style=CommandFrame]
\begin{minted}{python}
# Creating conda environment
> conda create -n Video2Metadata python=3.7
> conda activate Video2Metadata

# Install spaCy with NeuralCoref 
> cd Libraries
> git clone \
  https://github.com/huggingface/neuralcoref.git
> cd neuralcoref
> pip install -r requirements.txt
> pip install -e .
> cd ../../

# Download the spaCy language model
> python -m spacy download en_core_web_lg
# Install WordNet
> conda install -c anaconda nltk

# Only necessary when you want to query categories 
# from the YouTube Data API
> conda install -c conda-forge \ 
  google-api-python-client
\end{minted}
\end{mdframed}
\vspace{2mm}

\noindent If errors occur when installing spaCy with NeuralCoref, then run the following commands: 

\vspace{1mm}
\begin{mdframed}[style=CommandFrame]
\begin{minted}{python}
# Remove and create conda environment
> conda deactivate
> conda env remove -n Video2Metadata
> conda create -n Video2Metadata python=3.7
> conda activate Video2Metadata

# Install spaCy with NeuralCoref, and download
# the spaCy language model
> pip install spacy==2.1.0
> pip install neuralcoref
> python -m spacy download en_core_web_lg

# Install WordNet
> conda install -c anaconda nltk

# Only necessary when you want to query categories 
# from the YouTube Data API
> conda install -c conda-forge \ 
  google-api-python-client
\end{minted}
\end{mdframed}
\vspace{1mm}

\noindent With the first sequence of commands, NeuralCoref is installed from source, while the second command sequence installs NeuralCoref via \texttt{pip}. NeuralCoref can be installed via \texttt{pip} only when spaCy version is 2.1.0 or lower. With spaCy 2.1.0, however, the language parser operates much slower. Therefore, the first installation process is to be preferred.

\subsubsection*{\textbf{Files and Usage.}} \ \\
We now explain the repository's files and how they can be used to extract semantic metadata and to evaluate the extraction methods of our framework.\\

\noindent \texttt{- example\_extraction\_from\_text.py} \\
\noindent Run this program to extract and print video-level entities, properties, and video-level relations from a given input text. Text can be passed with the \texttt{text} option. Example:
\vspace{1mm}
\begin{mdframed}[style=SmallCommandFrame]
\begin{minted}{bash}
> python ./example_extraction_from_text.py \ 
  --text "A man is standing in front of a \ 
  fridge. He opens it and takes out a red glass."
\end{minted}
\end{mdframed}
\vspace{1mm}

\noindent \texttt{- examples.py} \\
\noindent To test the entity, property, and relation extraction methods on given captioned events, you can edit the script's examples at own will. Running this script with the following command will print the extracted video-level and event-level entities, entity-property pairs, and video-level and event-level relations:
\vspace{1mm}
\begin{mdframed}[style=SmallCommandFrame]
\begin{minted}{bash}
> python example.py
\end{minted}
\end{mdframed}
\vspace{1mm}

\noindent \texttt{- data\_dvc\_output/} \\
\noindent As mentioned above, we do not provide any source code for the DVC models. Instead, we generated captioned events for all ActivityNet Captions train and validation videos with both models and saved those to JSON files. This directory contains the generated (distinct) captioned events for $|E|$ set to 10, 25, 50, 100, and $|dist(E)|$ set to 1, 3, 10, 25. \texttt{MT\_train\_and\_val\_10\_no\_dup.json}, e.g., contains 10 distinct captioned events per ActivityNet Captions train and validation video generated with the MT model.\\

\noindent \texttt{- dataset\_activity\_net\_captions/} \\
\noindent Contains the ActivityNet Captions dataset\footnote{ActivityNet Captions: \url{https://cs.stanford.edu/people/ranjaykrishna/densevid/}.}, which is used for training of the DVC models and generating the gold standards for entity, property, and relation extraction.\\

\noindent \texttt{- Libraries/} \\
\noindent This directory contains Python files regarding the implementation of the semantic metadata extraction methods of Section~\ref{sec:method}, i.e., the algorithms for entity, property, and relation extraction (\texttt{entities\_lib.py}, \texttt{relations\_lib.py}), class definitions of entities, properties, and relations (\texttt{entity.py}, \texttt{entity\_property.py}, \texttt{relation.py}), a file for building the spaCy language parser (\texttt{nlp\_lib.py}), and a file that contains logic regarding WordNet (\texttt{wordnet\_lib.py}).\\

\noindent \texttt{- Semantic\_Metadata\_Extraction/} \\
\noindent \texttt{Semantic\_Metadata\_Extraction/scripts/} contains all scripts for generating and evaluating the results for entity, property, and relation extraction presented in this work. Among others, the most important scripts are:\\

\noindent 1) \texttt{extract\_sm.py}: Extracts entities, entity-property pairs, and relations from the input captioned events. All results are saved to \texttt{Semantic\_Metadata\_Extraction/output\_data/}. Using this script, the gold standards for entities, properties, and relations (see Section~\ref{sec:experiments/datasets}) can be generated using the following command:

\vspace{1mm}
\begin{mdframed}[style=SmallCommandFrame]
\begin{minted}{bash}
> python extract_sm.py --type gt --id GT
\end{minted}
\end{mdframed}
\vspace{1mm}

\noindent To extract semantic metadata from generated captioned events, e.g., from 10 distinct captioned events generated with the PDVC model, the following command is used: 

\vspace{1mm}
\begin{mdframed}[style=SmallCommandFrame]
\begin{minted}{bash}
> python extract_sm.py --type submission \ 
  --submission ./../../data_dvc_output/PDVC_ \ 
  train_and_val_10_no_dup.json --id PDVC_10_no_dup
\end{minted}
\end{mdframed}
\vspace{1mm}

\noindent 2) \texttt{evaluate\_event\_entities.py}: After semantic metadata for entities, properties, and relations is now generated, we can evaluate all extraction methods. More generally, we can evaluate the capability of our framework for entity, property, and relation extraction. The performance for event-level entity extraction is evaluated using this script. By specifying the gold standard, the submission file, and the ActivityNet Captions set(s) on which to evaluate, we can measure precision, recall, and F1 score performances of our framework. Example:

\vspace{1mm}
\begin{mdframed}[style=SmallCommandFrame]
\begin{minted}{bash}
> python evaluate_event_entities.py --gt \ 
  ./../output_data/sm_GT.json --submission \ 
  ./../output_data/sm_MT_10.json --split val
\end{minted}
\end{mdframed}
\vspace{1mm}

\noindent 3) \texttt{evaluate\_event\_relations.py}: Evaluate event-level relation extraction. Example:

\vspace{1mm}
\begin{mdframed}[style=SmallCommandFrame]
\begin{minted}{bash}
> python evaluate_event_relations.py --gt \
  ./../output_data/sm_GT.json --submission \
  ./../output_data/sm_PDVC_25.json --split val
\end{minted}
\end{mdframed}
\vspace{1mm}

\newpage
\noindent 4) \texttt{evaluate\_properties.py}: Evaluate property extraction. Example:

\vspace{1mm}
\begin{mdframed}[style=SmallCommandFrame]
\begin{minted}{bash}
> python evaluate_properties.py --gt \ 
  ./../output_data/sm_GT.json --submission \
  ./../output_data/sm_PDVC_25_no_dup.json \ 
  --split val
\end{minted}
\end{mdframed}
\vspace{1mm}

\noindent 5) \texttt{evaluate\_video\_entities.py}: Evaluate video-level entity extraction. Example:

\vspace{1mm}
\begin{mdframed}[style=SmallCommandFrame]
\begin{minted}{bash}
> python evaluate_video_entities.py --gt \ 
  ./../output_data/sm_GT.json --submission \ 
  ./../output_data/sm_PDVC_10_no_dup.json \ 
  --split val
\end{minted}
\end{mdframed}
\vspace{1mm}

\noindent 6) \texttt{evaluate\_video\_relations.py}: Evaluate video-level relation extraction. Example:

\vspace{1mm}
\begin{mdframed}[style=SmallCommandFrame]
\begin{minted}{bash}
> python evaluate_video_relations.py --gt \ 
  ./../output_data/sm_GT.json --submission \ 
  ./../output_data/sm_MT_3_no_dup.json \ 
  --split val
\end{minted}
\end{mdframed}
\vspace{1mm}

\noindent 7) \texttt{build\_frequent\_entities.py}: Needed to evaluate video-level entities. Calculates the frequency of entities in the ActivityNet Captions dataset (see Table~\ref{tab:statistics_entity_frequency_threshold}).

\vspace{1mm}
\begin{mdframed}[style=SmallCommandFrame]
\begin{minted}{bash}
> python build_frequent_entities.py
\end{minted}
\end{mdframed}
\ \\

\noindent \texttt{- dataset\_activity\_net\_entities/} \\
\noindent Contains the ActivityNet-Entities dataset\footnote{ActivityNet-Entities: \url{https://github.com/facebookresearch/ActivityNet-Entities}.}, which is used in this work to analyse how many entities that are extracted by our framework for ActivityNet Captions videos are actually not visible in the video (see Section~\ref{sec:discussion/threads}).\\

\noindent \texttt{- dataset\_classification/} \\
\noindent Contains our dataset for video classification, i.e., the video categories of ActivityNet Captions videos, queried from the YouTube Data API, and the train, validation, and test splits (see Sec.~\ref{sec:experiments/datasets}).\\

\noindent \texttt{- Text\_Classification/} \\
\noindent As opposed to the methods for entity, property, and relation extraction, the text classification method of our framework is implemented and evaluated in \texttt{classify\_text\_with\_bert.ipynb}, i.e., a single Jupyter Notebook. Note that we ran the experiments for text classification in Google Colab\footnote{Google Colab: \url{https://colab.research.google.com/}.}. Therefore, to run the experiments on a local machine, minor changes to the code are necessary. This concerns the locations of used files (classification dataset, generated captioned events), and also the installation of dependencies. The text classification method requires the installation of dependencies different from those named above and is handled in the Jupyter Notebook.\\

\noindent \texttt{- mini\_gold\_standards/} \\
\noindent Contains the manually annotated gold standard of 25 ActivityNet Captions videos with the video-level entities, entity-property pairs, and video-level relations that we expect the semantic metadata extraction methods to extract from captioned events (see Sec.~\ref{sec:discussion/threads}).
